# Supplementary material for: PixelGen: Rethinking Embedded Camera Systems
Source: arXiv:2402.03390 source file (2024-02-04)
Supplement: Supplementary file 1 [file appendix.tex]

\section{Appendix}
% \textbf{\hl{Add schematic of the pixelsense here, also highlight individual blocks with their corresponding application.}}

\fakepar{Using Robot to Visualize Audio and RF Emission} The use case for the diffusion model can be extended further to visualize non-visible spectrum such as audio and radio frequency (RF). In this setup, we introduced another interface, an autonomous robot equipped with a camera and audio and RF emission sensors. The robot can move around the floor and record the audio and RF emissions of each of the rooms. After collecting the emission data, the robot will proceed to a location that can capture a wide-angle photo of the rooms. The photo and the emission data will then be sent to the edge device that will interface with the multi-modal model that will mark the position of the rooms and indicate the strength of audio and RF emission. This produces 3 layers of image set: original image, audio emission image, and RF emission image. These layers will be sent to Control Net to be pre-processed for combination. 

\fakepar{Motion Blur Visualization}
We are collecting the acceleration information from the LSM9DS1 inertial module. Considering the movement of our robot is mostly in the lab (2D space), we are focused on the overall acceleration of x and y direction. The maximum acceleration of the robot should be around 5~$m^2/s$ and we are using motion blur in the photo to visualize the acceleration level. There are three levels: no motion blur (should be the same as a good quality realistic image), slight motion blur, and obvious motion blur. Based on the robot speed and camera exposure, 2~$m^2/s$ can be used as a boundary for slight and obvious motion blur.

Here are some examples of prompts generated by GPT-4 after feeding the sensor values.

Ambient Light: 3196 Lux;
Temperature: 28.04 Celsius;
Humidity: 71.54 \%;
Pressure: 1003.64 hPa;
Wind Velocity: 0.0 m/s;
Acceleration: 3.8~$m^2/s$

Moderately bright, partly cloudy day with warm temperatures and a very moist, muggy atmosphere, no wind, indicating changing weather conditions, captured in a high-quality image with obvious motion blur, emphasizing a dynamic and active environment

Ambient Light: 3196 Lux;
Temperature: 28.04 Celsius;
Humidity: 71.54 \%;
Pressure: 1003.64 hPa;
Wind Velocity: 0.0 m/s;
Acceleration: 1.2~$m^2/s$

A warm, humid, and moderately bright day with partly cloudy skies, no wind, and slightly changing weather conditions, captured in a high-quality image with slight motion blur, conveying a sense of calmness and stillness in the environment.

Refer to image generated (motion blur).

\fakepar{Power Consumption}
1.Ambiq Apollo3 Blue SoC: 
typical voltage: 3.3V; 
low power as 6uA per MHz (less than 5mW); \\
https://ambiq.com/wp-content/uploads/2020/10/Apollo3-Blue-SoC-Datasheet.pdf 

2.Himax HM01B0: 
QVGA 30FPS (Typical) < 2mW; \\
https://www.himax.com.tw/products/cmos-image-sensor/always-on-vision-sensors/hm01b0/

3.Bosch BME280: 
typical voltage: 3.3V; 
average current when collecting three information (Temperature, Humidity, and Pressure): 3.6 µA @1Hz; \\
https://www.bosch-sensortec.com/media/boschsensortec/downloads/product\_flyer/bst-bme280-fl000.pdf

4.ROHM BH1750FVI: 
typical voltage: 3.0V; 
typical current: 0.12mA; \\
https://www.mouser.com/datasheet/2/348/bh1750fvi-e-186247.pdf

5. MSP430FR5969: 
typical voltage: 3.3V; 
typical current: 100$\mu$A; \\
https://www.ti.com/document-viewer/msp430fr5969/datasheet
